# Supplementary material for: A search for rare $B \rightarrow D \mu^+ \mu^-$ decays
Source: arXiv:2308.06162 source file (2024-02-26)
Supplement: Supplementary file 1 [file appendix.tex]

\appendix

\section{Correlation matrices}
\label{sec:appendix}
